# Supplementary material for: MATEX: A Distributed Framework for Transient Simulation of Power Distribution Networks
Source: arXiv:1511.04519 source file (2015-11-14)
Supplement: Supplementary file 1 [file appendix.tex]

\fontsize{9pt}{9pt}
This is supplemental material includes 
discussions of MATEX, 
mathematical deductions for I-MATEX posterior error term,
and figures for numerical results discussed in the paper.

\section{Discussions about MATEX and Traditional methods (TR, BE)}

MATEX stems from Krylov subspace based matrix exponential computation.
With accurate exponential calculation via Krylov subspace basis, it can reuse the basis to
carry adaptive time stepping along successive time spots (taking \emph{snapshots})
before hitting the next LTS.
The snapshot can be obtained as \emph{by-products} by scaling Hessenberg matrix 
and matrix exponential evaluation based on adaptive time stepping
techniques similar in MEXP \cite{Weng12_TCAD, Zhuang13_ASICON}.
In addition, MATEX benefits a lot from reusing factorized matrices, which come from
the very beginning of simulation, to generate
new Krylov subspace basis once reaching LTS.
%The LTS, GTS in the Fig. \ref{fig:input}, can be precomputed based on the provided input sources
%information and avoid communication among different computing nodes, 
There are no communication overhead during the transient computing,
rendering such framework 
be a good candidate computational problems for large scale computing techniques, e.g. 
MapReduce, Hadoop, %Mesos, 
Spark, etc., which now may scale to tens of thousands of nodes, 
to deal with large number of input sets.

Nevertheless, the major hinder of traditional methods are LTE due to the low order polynomial approximation, 
and incapability of reusing factorized matrices once changing $h$ (e.g. $C/h+G/2$ 
in Eqn. \ref{eqn:trap} need to be re-factorized for solving the linear system). 
Within each node, we still need to derive the transient solutions 
step by step along all time spots (GTS) with calculations, 
e.g. LU, Cholesky, 
or pairs of backward and forward substitutions. 
Therefore, to them, there is no benefit from such input transition decompositions.
Model order reduction techniques can be applied here, however, they are not full model simulation
and cannot control the error on-the-fly, which MATEX serves all the purposes. 

%\section{Circuit Solver Algorithm}

\section{Derivation of I-MATEX posterior error term}
Follow the residual concept \cite{Botchev2013}, 
we obtain the error approximation of I-MATEX in Eq. (\ref{eq:err_inverted_krylov}).
\begin{comment}
\begin{eqnarray}
\label{eq:err_rational_krylov}
\lVert \mbf r_m(h) \rVert 
=
\lVert \mbf v \rVert
\left |  
\frac{\mbf I - \gamma \mbf A_m}{\gamma} 
\tilde{h}_{m+1,m}
\mbf v_{m+1} 
\mbf e^T_m \mbf{\widetilde {H}}_m^{-1}  
%{ \phi( h\mbf{\wtd H_m})} 
 e^{ h\mbf{ H}_m} 
 \mbf e_1 \right |
\end{eqnarray}
\end{comment}

\begin{eqnarray}
\mbf r_m(h) & =&  \mbf A \mbf x_m(h) - \mbf x_m'  
 \nonumber
\\ \nonumber
&=& 
\lVert \mbf v \rVert \mbf A \mbf V_m e^{h\mbf {H'}_m^{-1}}
\mbf e_1 - 
\lVert \mbf v \rVert \mbf V_m \mbf {H'}^{-1}_m 
e^{h \mbf {H'}_m^{-1}} \mbf e_1 
\\ \nonumber
&=&
\lVert \mbf v \rVert (\mbf A \mbf V_m 
- \mbf V_m \mbf {H'}^{-1}_m) 
  e^{h \mbf {H'}_m^{-1}} \mbf e_1 
\\ \nonumber
&=&
-
  \lVert \mbf v  \rVert
 \mbf A h'_{m+1,m} \mbf v_{m+1} \mbf e_m^{T} 
\mbf {H'}^{-1}_m e^{h\mbf {H'}_m^{-1}} \mbf e_1
\end{eqnarray}

The error term for rational Krylov subspace based matrix 
exponential computation (R-MATEX) can be also found in \cite{Botchev2013}. 

%\section{Characteristics of R-MATEX}
\begin{comment}

In this section, we show the relation trends among Krylov subspace dimension ($m$),
time step size ($h$) and error ($Error$).
%\section{Error trend of rational Krylov subspace based matrix exponential } 
The error is defined as
\begin{eqnarray}
Error = |e^{h\mbf A}\mbf v - \mbf V_m e^{h\mbf H_m}\mbf e_1|
\\
\nonumber
\end{eqnarray}
where
$\mbf H_m$ = $\frac{\mbf I - \mbf {\wtd H}_m}{\gamma} $, 
and $\mbf A$ is a small matrix and computed by MATLAB $expm$ function, which is the baseline for accuracy. 

\section{Error vs. time step ($h$) and dimension of Krylov subspace basis ($m$)}
Fig. \ref{fig:h_m} shows when time step $h$ increases, the error actually is reduced
(fixed  $\gamma = 10^{-12}$). 
The reason was mentioned in \cite{Van06}.
The longer time step R-MATEX uses, 
the more dominating role first smallest magnitude eigenvalues play, which 
are well captured by our rational Krylov subspace-based method.
In our MATEX, this is very crucial elements making us to do time stepping as large as possible.
That is why we can use the formula in the line 15 of Alg. \ref{algo:ckt_solver}.
\begin{figure}[h]
    \centering
    \includegraphics[ width=3.4in]{./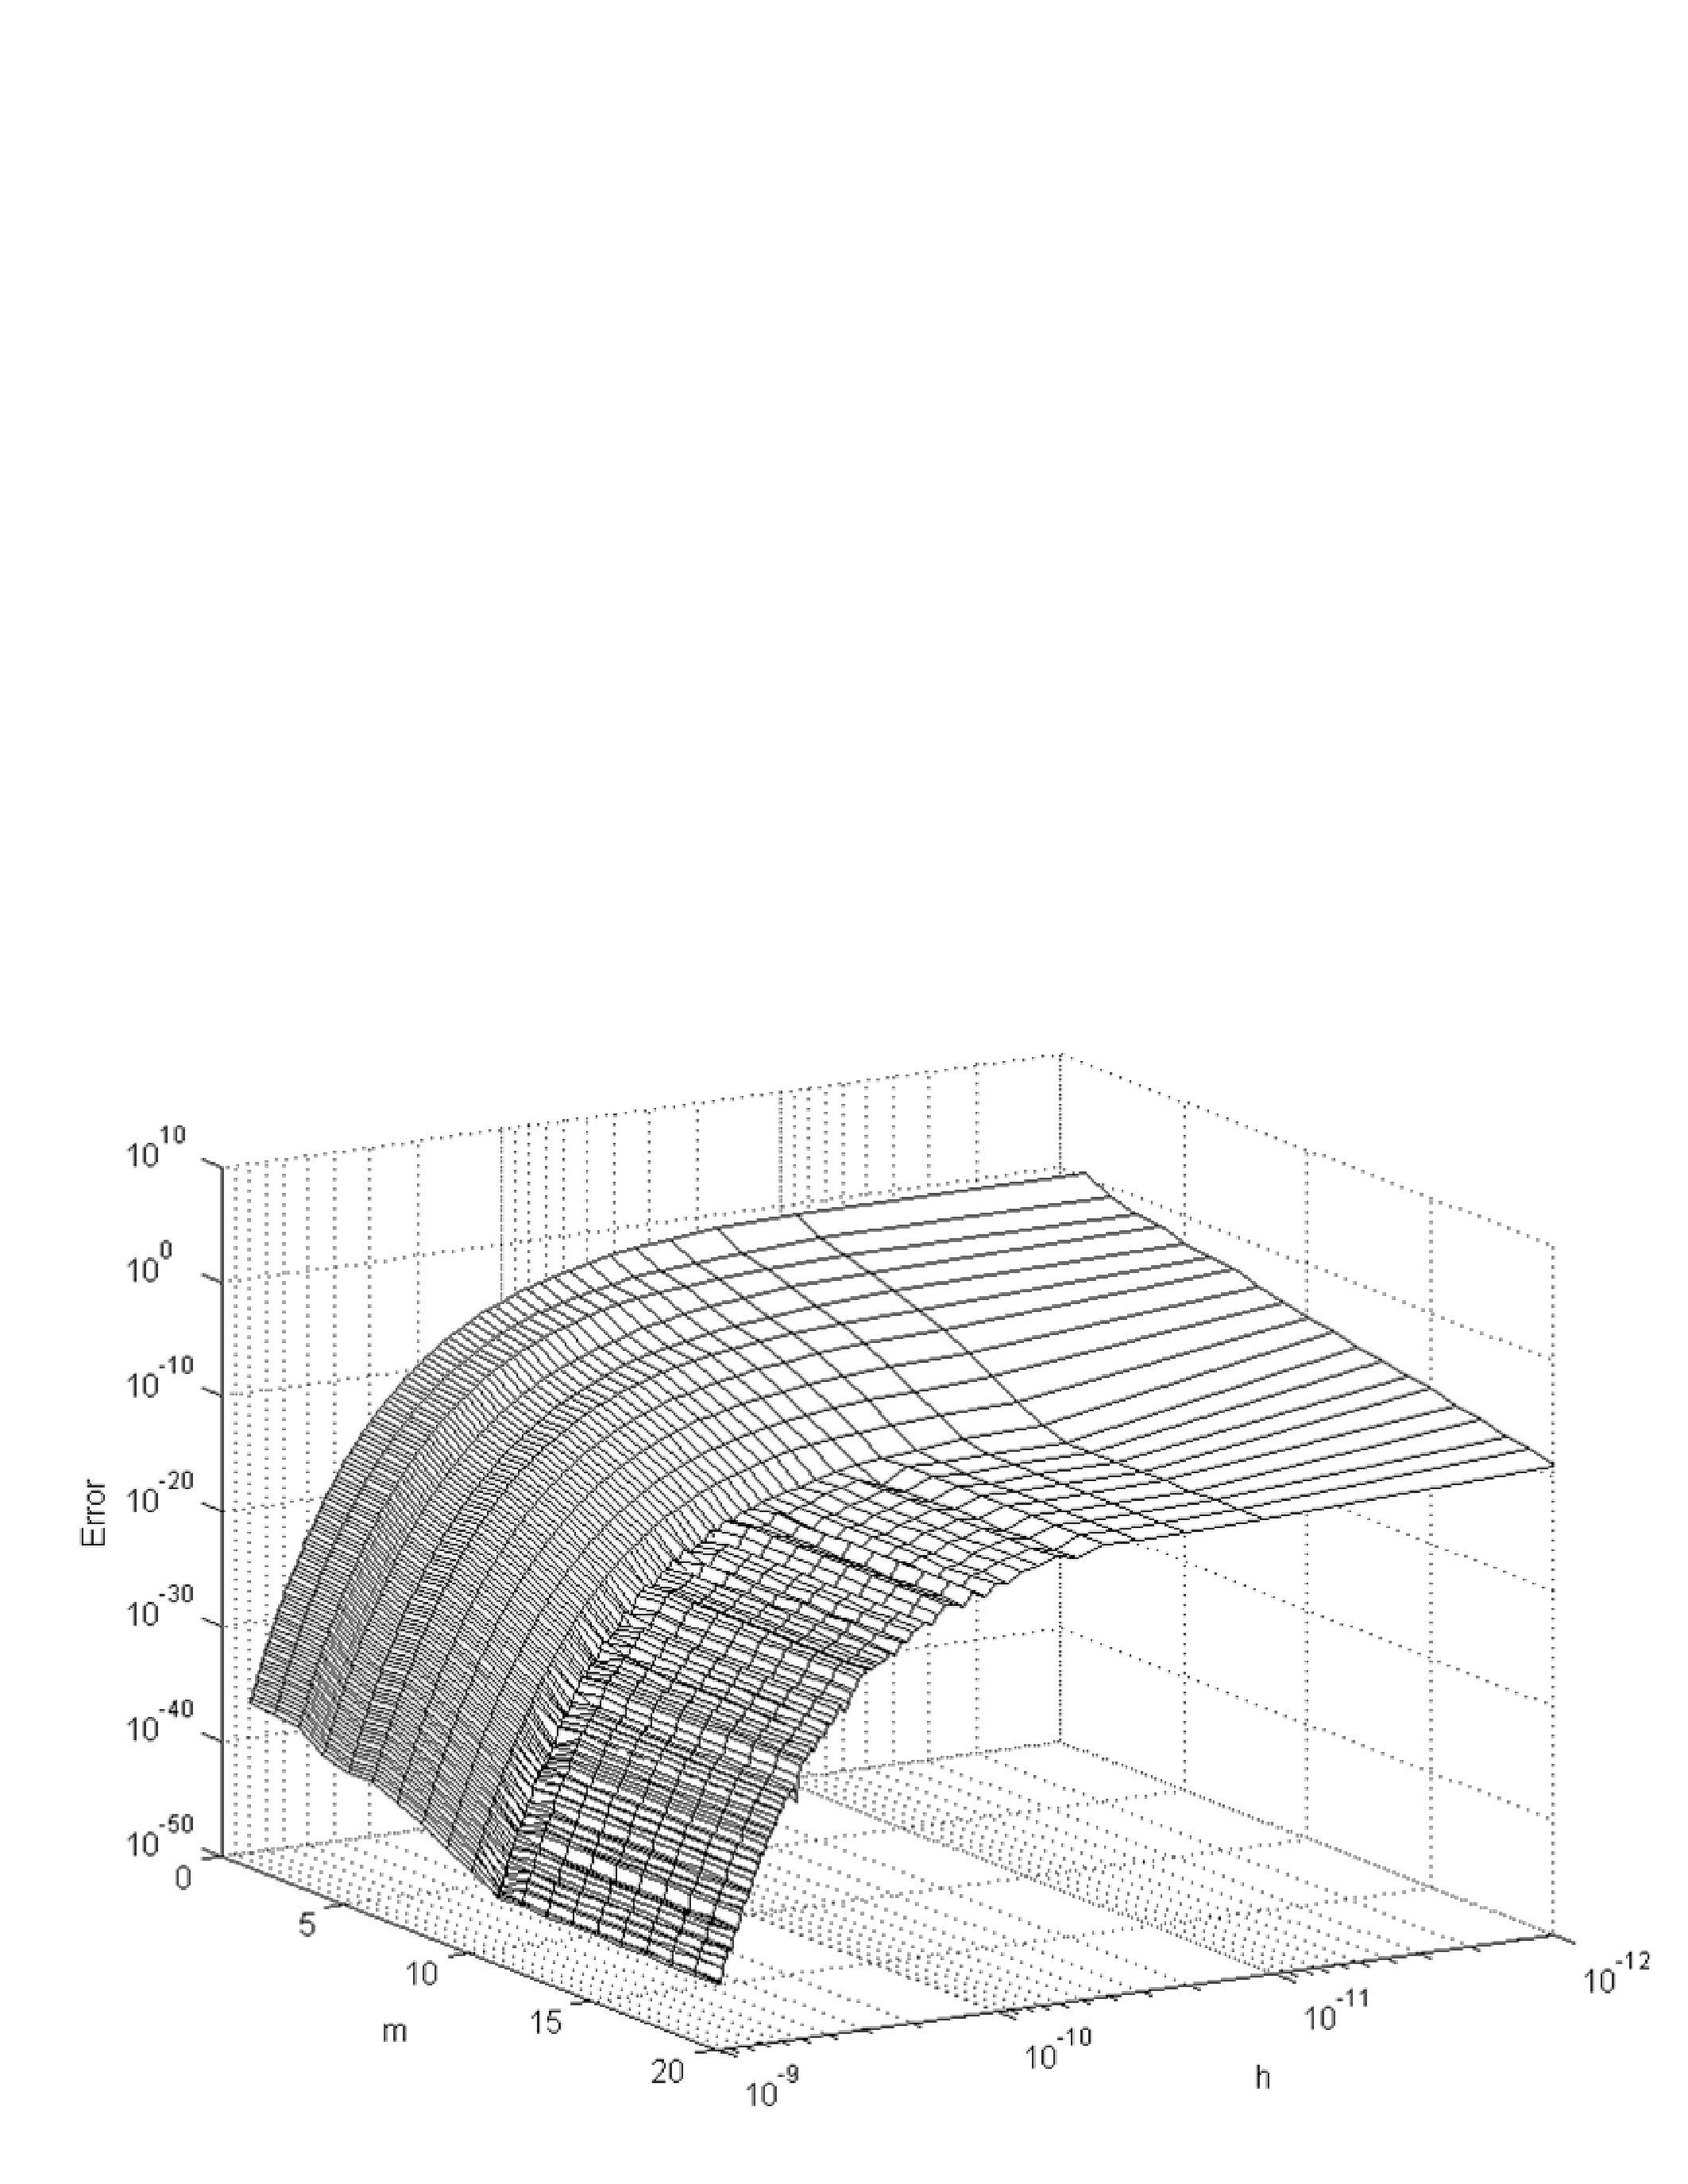}
    \caption{$|e^{h\mbf A}\mbf v - \mbf V_m e^{h\mbf H_m}\mbf e_1|$
    vs. time step $h$ and dimension of rational Krylov subspace basis (m)}
    \label{fig:h_m}
\end{figure}
\section{Error vs. $\gamma$ and dimension of Krylov subspace basis ($m$)}
\end{comment}
\section{Error vs. $\gamma$ and dimension of Krylov subspace basis ($m$)}
%We show the relation trends among Krylov subspace dimension ($m$) and $\gam error ($Error$).
%\section{Error trend of rational Krylov subspace based matrix exponential } 
Fig. \ref{fig:gamma_m} shows that, the error is not sensitive to the change of $\gamma$, 
where time step is fixed  at $h=100ps$. 
The error is defined as
\begin{eqnarray}
Error = |e^{h\mbf A}\mbf v - \mbf V_m e^{h\mbf H_m}\mbf e_1|
\nonumber
\end{eqnarray}
where
$\mbf H_m$ = $\frac{\mbf I - \mbf {\wtd H}_m}{\gamma} $, 
and $\mbf A$ is a small matrix and computed by MATLAB $expm$ function, which is the baseline for accuracy. 
\begin{figure}[h]
    \centering
    \includegraphics[width=3.4in]{./figs/gamma_m.eps}
    \caption{$|e^{h\mbf A}\mbf v - \mbf V_m e^{h\mbf H_m}\mbf e_1|$ vs. $\gamma$ and 
    dimension  of rational Krylov subspace basis ($m$). 
    Sweep $\gamma$ up to $10^{-9}$; 
    $m$ is from 1 to 10. When $m>5$, the error is very small (below $10^{-10}$). 
    That flat zone also shows R-MATEX is not sensitive to $\gamma$.}
    \label{fig:gamma_m}
\end{figure}
The same phenomena was found in \cite{Van06}.
Therefore, in our power grid simulation, we set $\gamma$  among the step sizes.

\section{IBMPG6T waveform}
To illustrate our adaptive stepping R-MATEX, 
we show the result from ibmpg6t (Fig. \ref{fig:result_ibmpg6t}). 
The star points are via R-MATEX. The star points are connected via piecewise segments. 
Even R-MATEX jumps large, it can still get accurate solution 
due to its high order polynomial approximation.
The TR and Solution (from IBM Power Grid Benchmark) are shown together.
\begin{figure}[h]
    \centering
    \includegraphics[width=3.5in]{./figs/result_ibmpg6t.eps}
    \caption{Result of ibmpg6t, the star points are calculated via R-MATEX. 
    It is observed that non-uniform time steps by the adaptive stepping of R-MATEX
    along the time span [$0s,10^{-8}s$].}
    \label{fig:result_ibmpg6t}
\end{figure}
