# Supplementary material for: MATEX: A Distributed Framework for Transient Simulation of Power Distribution Networks
Source: arXiv:1511.04519 source file (2015-11-14)
Supplement: Supplementary file 2 [file appendix_v1.tex]

%\onecolumn

\fontsize{9pt}{9pt}
This is supplemental material includes more detailed figures for numerical results 
and mathematical deductions for MATEX's circuit solver discussed in the paper.

\section{Circuit Solver Algorithm}

\begin{algorithm}
\label{algo:ckt_solver}
%\caption{Arnoldi process in Matrix Exponential-Based Circuit Simulation with Krylov subspace Method}
\caption{Circuit Solver Algorithm at MATEX Slave Node}
%$\rm K_m(\mbf X_1^{-1}\mbf X_2, \mbf v)$} %~\cite{Weng12_TCAD, Weng12_ICCAD}}
\KwIn{ LTS, GTS, Circuit }
%\KwOut{ $\mbf V_m, \mbf H_m,  m$ }
\KwOut{ local solution $\mbf x$ along GTS }
    {   
%	[$\mbf L, \mbf U$]=LU($\mbf X_1$)\\
%	Normalize the intial vector 
	$t=T_{start}$\;
	$[\mbf x(t), \mbf y(t)] = local\_DC\_analysis$\; 
	$[\mbf L,\mbf U] = \text{LU\_Decompose}( \mbf C+\gamma \mbf G)$\;
	\While { $t \leq T_{end}$}
	{
	Compute maximum allowed step size $h$ based on GTS, and update $\mbf y(t)$\;
	\If{$t \in $ LTS}
	{
	// Reach LTS and update the $\mbf V_m, \mbf H_m, \mbf v$\;
	$[ \mbf y(t+h), \mbf V_m, \mbf H_m,\mbf v 	]
	= \text{MATEX\_Arnoldi}(\mbf L,\mbf U,\mbf C, h, \mbf y(t), \epsilon )$ \;
	Update $\mbf x(t +h) $ based on Eq. (\ref{eqn:new_exact})\; 
	$lts = t$\;
	}
	\Else{
%	    \For  {$s_i \in (t_i + h,t_{i+1}]$}
	    {
	    // Take snapshots by reusing $\mbf V_m , \mbf H_m, \mbf v$ \;
	    $h = t - lts$\;
	    $\mbf y(t+h) = \lVert \mbf v \rVert \mbf {V_m} e^{h \mbf H_m} \mbf e_1 $\;
	Update $\mbf x(t +h) $ based on Eq. (\ref{eqn:new_exact})\; 
	%$\lVert r_m(h) \rVert  =  \lVert \mbf v \rVert \left| h_{m+1,m} e_m^T e^{h\mbf H_m} e_1 \right|$
	    }
	}
	$t= t+h$\;
	}
    }
\end{algorithm}

\subsection{Derivation of I-MATEX posterior error term}

Follow the residue concept \cite{Botchev2013},
we obtain the error approximation in Eq. (\ref{eq:err_inverted_krylov})

\begin{comment}
\begin{eqnarray}
\label{eq:err_rational_krylov}
\lVert \mbf r_m(h) \rVert 
=
\lVert \mbf v \rVert
\left |  
\frac{\mbf I - \gamma \mbf A_m}{\gamma} 
\tilde{h}_{m+1,m}
\mbf v_{m+1} 
\mbf e^T_m \mbf{\widetilde {H}}_m^{-1}  
%{ \phi( h\mbf{\wtd H_m})} 
 e^{ h\mbf{ H}_m} 
 \mbf e_1 \right |
\end{eqnarray}
\end{comment}

\begin{eqnarray}
\mbf r_m(h) & =&  \mbf A \mbf x_m(h) - \mbf x_m'  
 \nonumber
\\ \nonumber
&=& 
\lVert \mbf v \rVert \mbf A \mbf V_m e^{h\mbf {H'}_m^{-1}}
\mbf e_1 - 
\lVert \mbf v \rVert \mbf V_m \mbf {H'}^{-1}_m 
e^{h \mbf {H'}_m^{-1}} \mbf e_1 
\\ \nonumber
&=&
\lVert \mbf v \rVert (\mbf A \mbf V_m 
- \mbf V_m \mbf {H'}^{-1}_m) 
  e^{h \mbf {H'}_m^{-1}} \mbf e_1 
\\ \nonumber
&=&
-
  \lVert \mbf v  \rVert
 \mbf A h'_{m+1,m} \mbf v_{m+1} \mbf e_m^{T} 
\mbf {H'}^{-1}_m e^{h\mbf {H'}_m^{-1}} \mbf e_1
\end{eqnarray}

\section{Characteristics of R-MATEX}
In this section, we show the relation trends among Krylov subspace dimesion ($m$),
time step size ($h$) and error ($Error$).
%\section{Error trend of rational Krylov subspace based matrix exponential } 
The error is defined as
\begin{eqnarray}
Error = |e^{h\mbf A}\mbf v - \mbf V_m e^{h\mbf H_m}\mbf e_1|
\end{eqnarray}
where $\mbf A$ is a small matrix and computed by MATLAB $expm$ function, which is the baseline for accuracy. 
$\mbf H_m$ = $\frac{\mbf I - \mbf {\wtd H}_m}{\gamma} $.

\subsection{Error vs. time step ($h$) and dimension of Krylov subspace basis ($m$)}
Fig. \ref{fig:h_m} shows when time step $h$ increases, the error actually is reduced
(fixed  $\gamma = 10^{-12}$). 
The reason was mentioned in \cite{Van06}.
The longer time step R-MATEX uses, 
the more dominating role first smallest magnitude eigenvalues play, which 
are well captured by our rational Krylov subspace-based method.
In our MATEX, this is very crucial elements making us to do time stepping as large as possible.
\begin{figure}[h]
    \centering
    \includegraphics[ width=3.4in]{./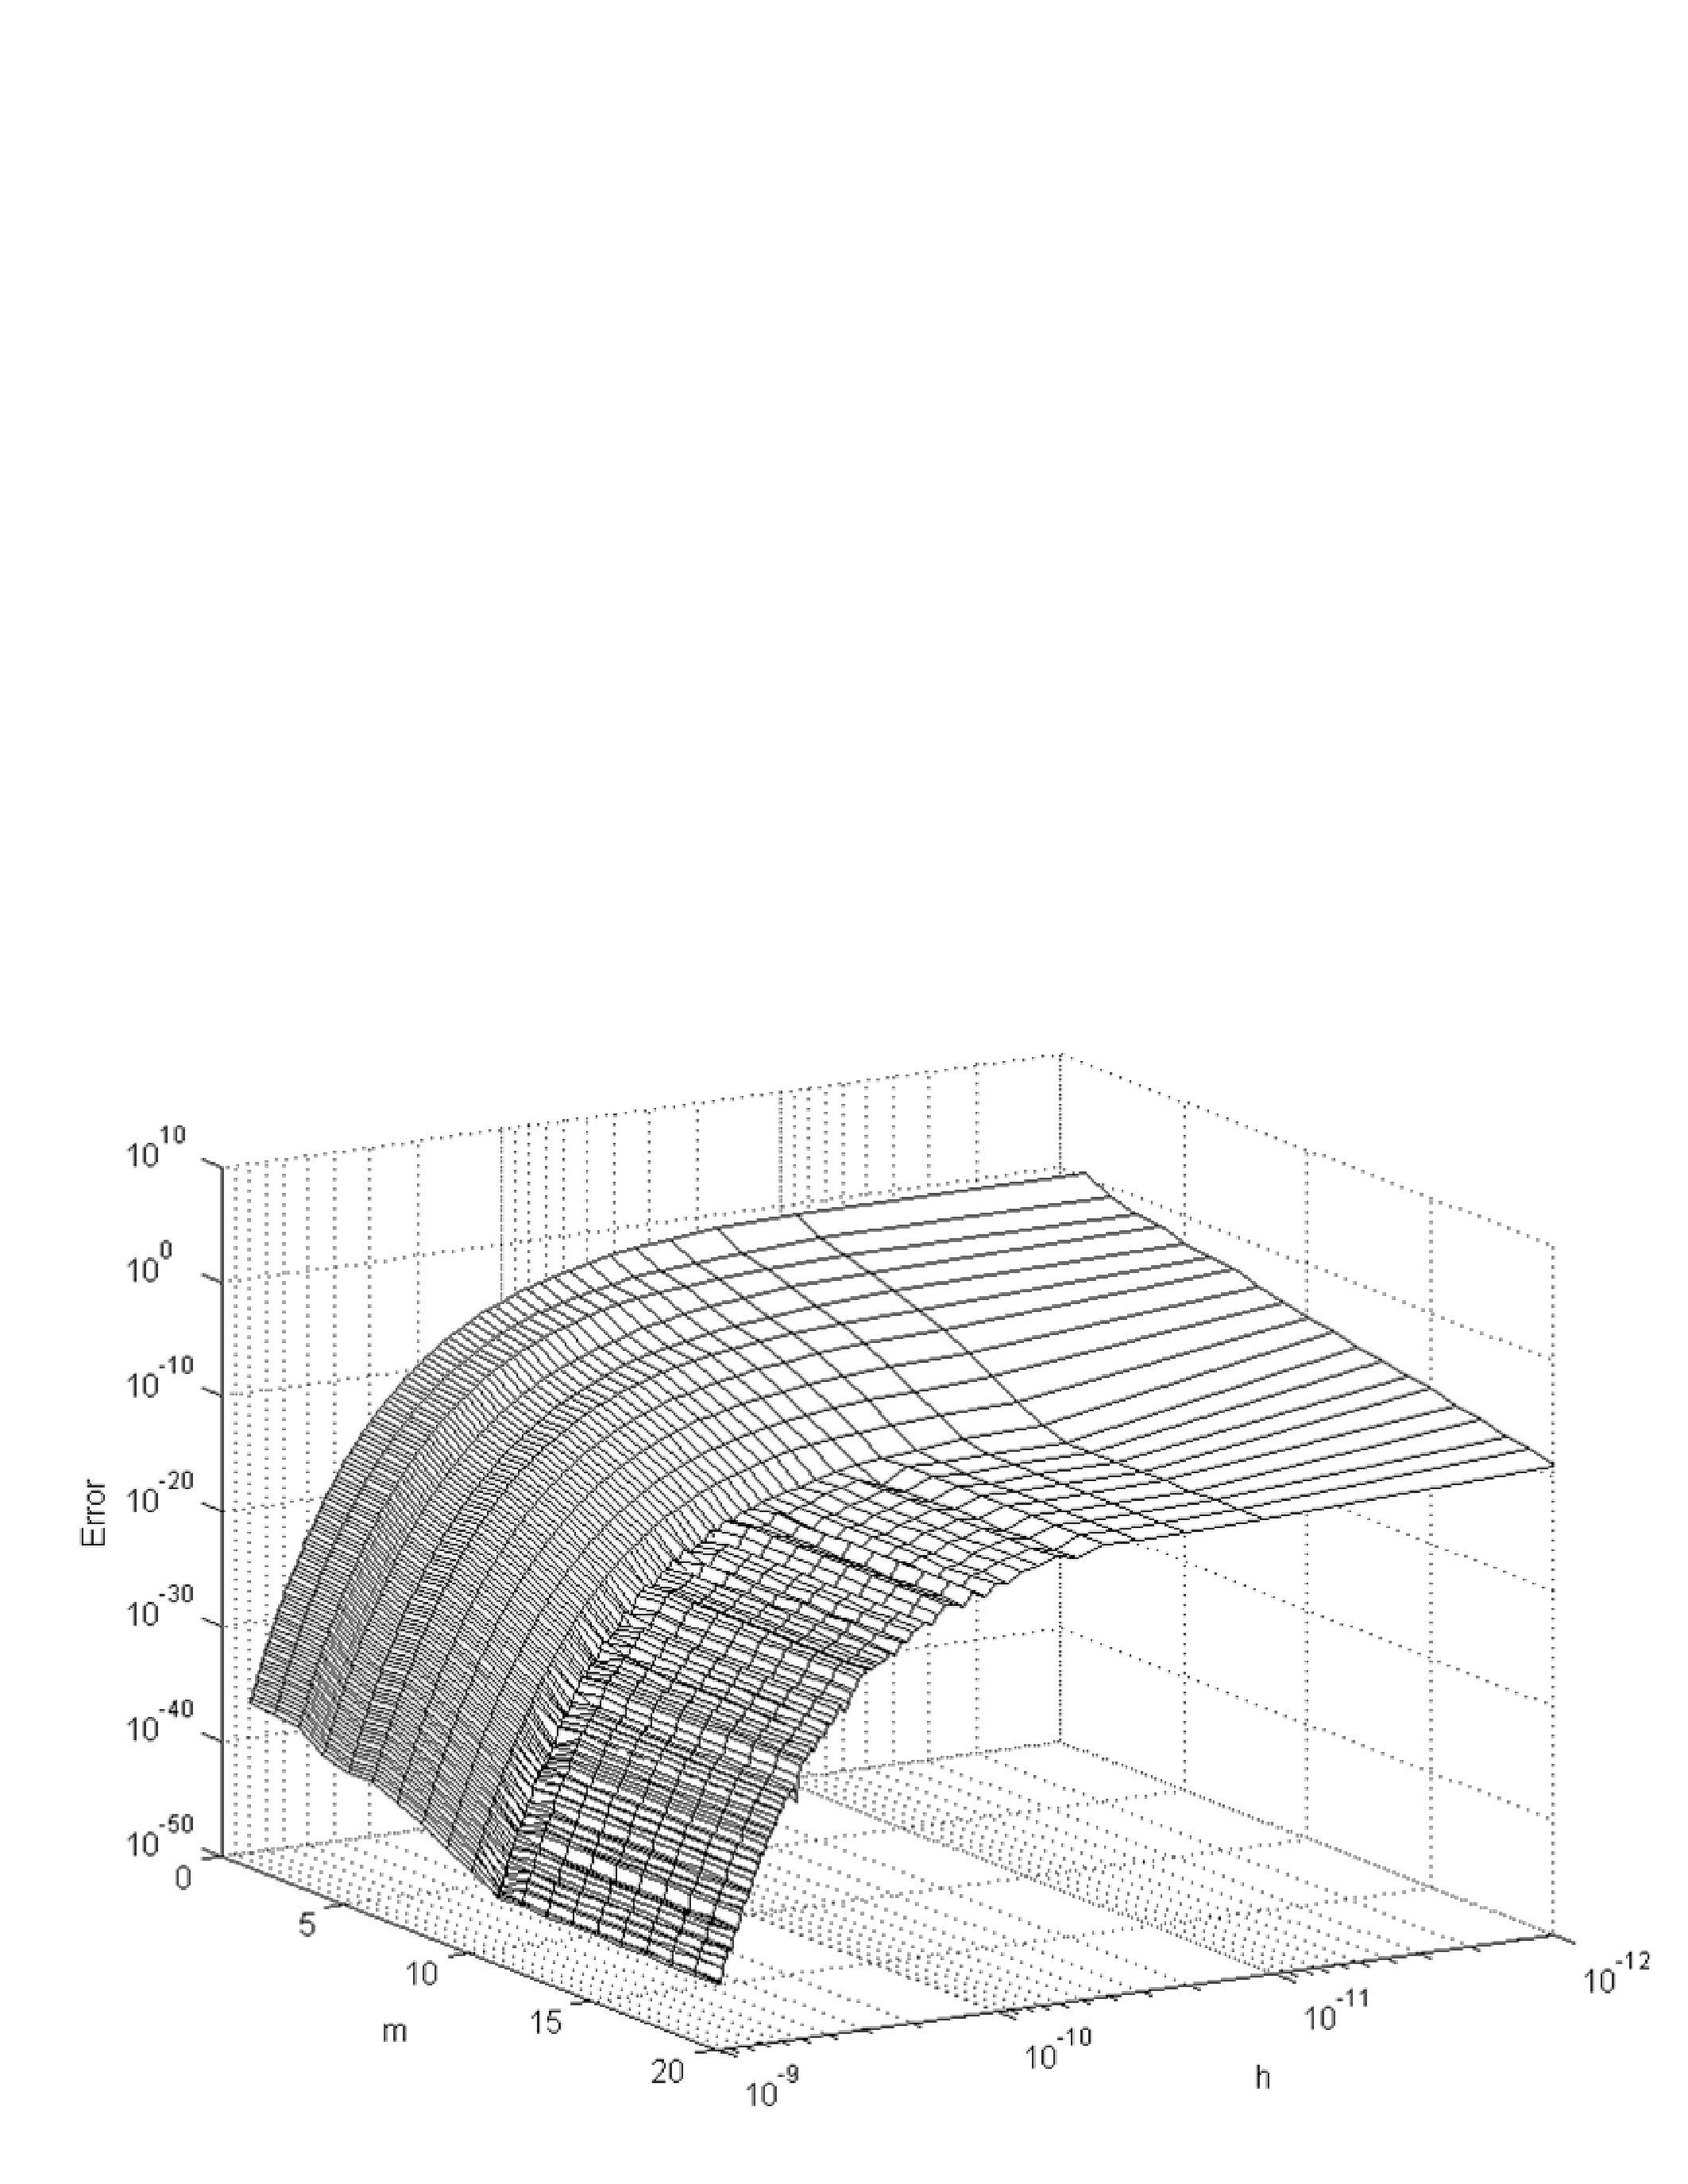}
    \caption{$|e^{h\mbf A}\mbf v - \mbf V_m e^{h\mbf H_m}\mbf e_1|$
    vs. time step $h$ and dimension of rational Krylov subspace basis (m)}
    \label{fig:h_m}
\end{figure}

\subsection{Error vs. $\gamma$ and dimension of Krylov subspace basis ($m$)}

Fig. \ref{fig:gamma_m} shows that, the error is not sensitive to the change of $\gamma$, 
where time step is fixed  at $h=100ps$. 
The same phenomena was found in \cite{Van06}.
\begin{figure}[h]
    \centering
    \includegraphics[width=3.4in]{./figs/gamma_m.eps}
    \caption{$|e^{h\mbf A}\mbf v - \mbf V_m e^{h\mbf H_m}\mbf e_1|$ vs. $\gamma$ and 
    dimension  of rational Krylov subspace basis ($m$)}
    \label{fig:gamma_m}
\end{figure}

Therefore, in our power grid simulation, we set $\gamma$  among the step sizes.

\subsection{IBMPG6T}
To illustrate our adaptive stepping method in R-MATEX, 
we show the result from ibmpg6t (Fig. \ref{fig:result_ibmpg6t}). 
The star points are via R-MATEX. The waveform is connected via piecewise segments. 
Even R-MATEX may jumps large, it can still get accurate enough solutions.
The TR and Solution (from IBM Power Grid Benchmark) are shown together.

\begin{figure}[h]
    \centering
    \includegraphics[width=3.5in]{./figs/result_ibmpg6t.eps}
    \caption{Result of ibmpg6t, the star points are calulated via R-MATEX. 
    It is observed that non-uniform time steps by the adaptive stepping of R-MATEX
    along the time span [$0s,10^{-8}s$].}
    \label{fig:result_ibmpg6t}
\end{figure}

The large time stepping without factorization of matrices brings MATEX efficiency
to trade Krylov subspace for pairs of backward and foward substitutions in TR with fixed time step.
